# Supplementary material for: Structure-Preserving Transformation: Generating Diverse and Transferable Adversarial Examples
Source: arXiv:1809.02786 source file (2018-12-22)
Supplement: Supplementary file 1 [file appendix.tex]

\section{Appendix}

\begin{table*}[t]
\centering
 \caption{Prediction statistics of different models for SPT adversarial examples on the MNIST (top) and F-MNIST (bottom) datasets}
 \label{tab:pred_statistics} 
\begin{center}
\begin{tabular}{c c c c c c c c c c c }
\toprule
Target  & 0 & 1 & 2 & 3 & 4 & 5 & 6 & 7 & 8 & 9\\
\hline
$C_{p}$ & 0.00\%& 0.00\%& 0.00\%& 0.00\%& 0.00\%& 0.00\%& 0.00\%& 0.00\%& \textbf{100\%}& 0.00\% \\

$C_{a0}$  & 0.00\%& 0.00\%& 0.00\%& 0.00\%& 0.00\%& 0.01\%& 0.00\%& 0.00\%& \textbf{99.99\%}& 0.00\% \\

$C_{a1}$& 0.00\%& 0.00\%& 0.00\%& \textbf{89.15\%}& 0.00\%& 0.01\%& 0.00\%& 0.00\%& \textbf{10.85}\%& 0.00\% \\
$C_{a2}$ & 0.06\%& 0.00\%& 0.00\%& 0.00\%& 0.00\%& \textbf{99.93\%}& 0.00\%& 0.00\%& 0.01\%& 0.00\% \\

$C_{a3}$ &  0.00\%& 0.00\%& \textbf{99.13\%}& 0.87\%& 0.00\%& 0.00\%& 0.00\%& 0.00\%& 0.00\%& 0.00\% \\ 
\bottomrule
\multicolumn{6}{c}{}\\
\multicolumn{6}{c}{}\\
\toprule
Target  & T-shirt/top & Trouser & Pullover & Dress & Coat & Sandal & Shirt & Sneaker & Bag & Ankle boot\\
\hline
$C_{p}$ & 0.00\%& 0.00\%& 0.00\%& 0.00\%& 0.00\%& 0.00\%& 0.00\%& 0.00\%& \textbf{100\%}& 0.00\% \\

$C_{a0}$ &  \textbf{37.03\%}& 4.54\%& 1.93\%& 0.71\%& 0.00\%& 9.28\%& 15.3\%& 0.01\%& \textbf{26.11\%}& 5.09\% \\

$C_{a1}$ &  0.00\%& 0.00\%& 0.00\%& 0.00\%& 0.00\%& 0.00\%& 0.02\%& 0.00\%& \textbf{99.49\%}& 0.49\% \\

$C_{a2}$ &  2.93\%& 15.49\%& 0.57\%& 0.08\%& 0.00\%& 2.94\%& 11.89\%& 0.00\%& \textbf{64.63\%}& 1.47\% \\

$C_{a3}$ &  0.00\%& 0.00\%& 0.00\%& 0.00\%& 0.00\%& 0.00\%& 0.26\%& 0.00\%& \textbf{99.74\%}& 0.00\% \\ 
\bottomrule
\end{tabular}
\end{center}
\end{table*}

\begin{table*}[p] 

\caption{Neural network architectures for classifiers used in experiments. $C_{a0}$ shares the same architecture as $C_{p}$, and only differs in the initialization of the weights.
}
\label{tab:archi}
\begin{center}
\begin{tabular}{c|c|c|c}
\toprule
$C_{p}$ , $C_{a0}$ & $C_{a1}$ & $C_{a2}$  & $C_{a3}$ \\
\hline
Conv(32, 5, 5, 1) & Conv(32, 4, 4, 1) & Conv(32, 3, 3, 1) & Conv(32, 3, 3, 1)\\
Relu & Relu & Relu & Relu\\
Max Pool(2, 2)& Max Pool(2, 2) & Max Pool(2, 2) & Max Pool(2, 2)\\
Conv(64, 5, 5, 1) & Conv(32, 4, 4, 1)& Conv(32, 3, 3, 1)& FC(1024)\\
Relu & Relu & Relu& Relu\\
Max Pool(2, 2) & Max Pool(2, 2) & Max Pool(2, 2) & Fc(512)\\
FC(1024) &  Conv(64, 4, 4, 1) &Conv(64, 3, 3, 1)& Relu\\
FC(10) + Softmax  & FC(1024) & FC(1024) & Fc(10) + Softmax\\
&FC(10) + Softmax & FC(10) + Softmax&\\
\hline
\end{tabular}
\end{center}

\end{table*}
%---------------------------------

\subsection{The Choice of Exponents of Power Functions}
In the experiments, %the SPT is assumed to be a linear combination of a number of power functions. T
the exponents $\gamma$ of the power functions in SPT are empirically set to  $\{0.04, 0.10, 0.20, 0.40, 0.67, 1.0, 1.5, 2.5, 5.0, 10.0, 25.0\}$. The underlying reason is that these basic functions could well reflect % We consider these 11 basic power function mainly base the 
different transformation intensities. % of different basic power function.
%These basic functions are plotted in 
(see Figure~\ref{fig:pow_law}). A power function with a larger $\gamma$ will generate a darker image and vise versa. 
%, they often make most pixels in the image dark, while for the power functions with small $\gamma$, they are more prone to be make image light. 
%------------------
\begin{figure}[h]
\centering
\includegraphics[height=2.5in,width=0.38\textwidth]{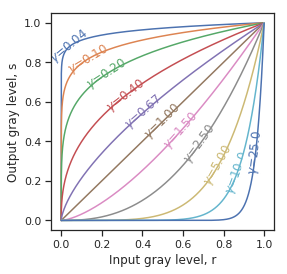}
\caption{the equation $s=cr^{\gamma}$ for various values of $\gamma$ }
\label{fig:pow_law}
\end{figure}
%-----------------
\smallskip

\subsection{Neural Network Architectures}
Details of the five network architectures used in the paper can be found in Table \ref{tab:archi}. In the table, Conv($m, k, k, s$) denotes a convolutional layer with $m$ feature maps, filter size $k \times k$, and stride $s$, Max Pool($n, n$) denotes a max pooling layer with filters of size $n \times n$, FC($m$) denotes a fully-connected layer with $m$ outputs, and ReLU denotes the Rectified Linear Unit activation function.
%----------------------------------archi------------------------------------

\subsection{Prediction Statistics for Adversarial Examples}
The prediction statistics for  white-box SPT adversarial examples are reported in Table~\ref{tab:pred_statistics}. Each row in the table records the percentage of SPT adversarial examples that are classified into each label %SPT adversarial examples classified
by a particular target model. The result shows that most adversarial examples are classified into the same class by any target model. 

\begin{figure*}[t]  
    \includegraphics{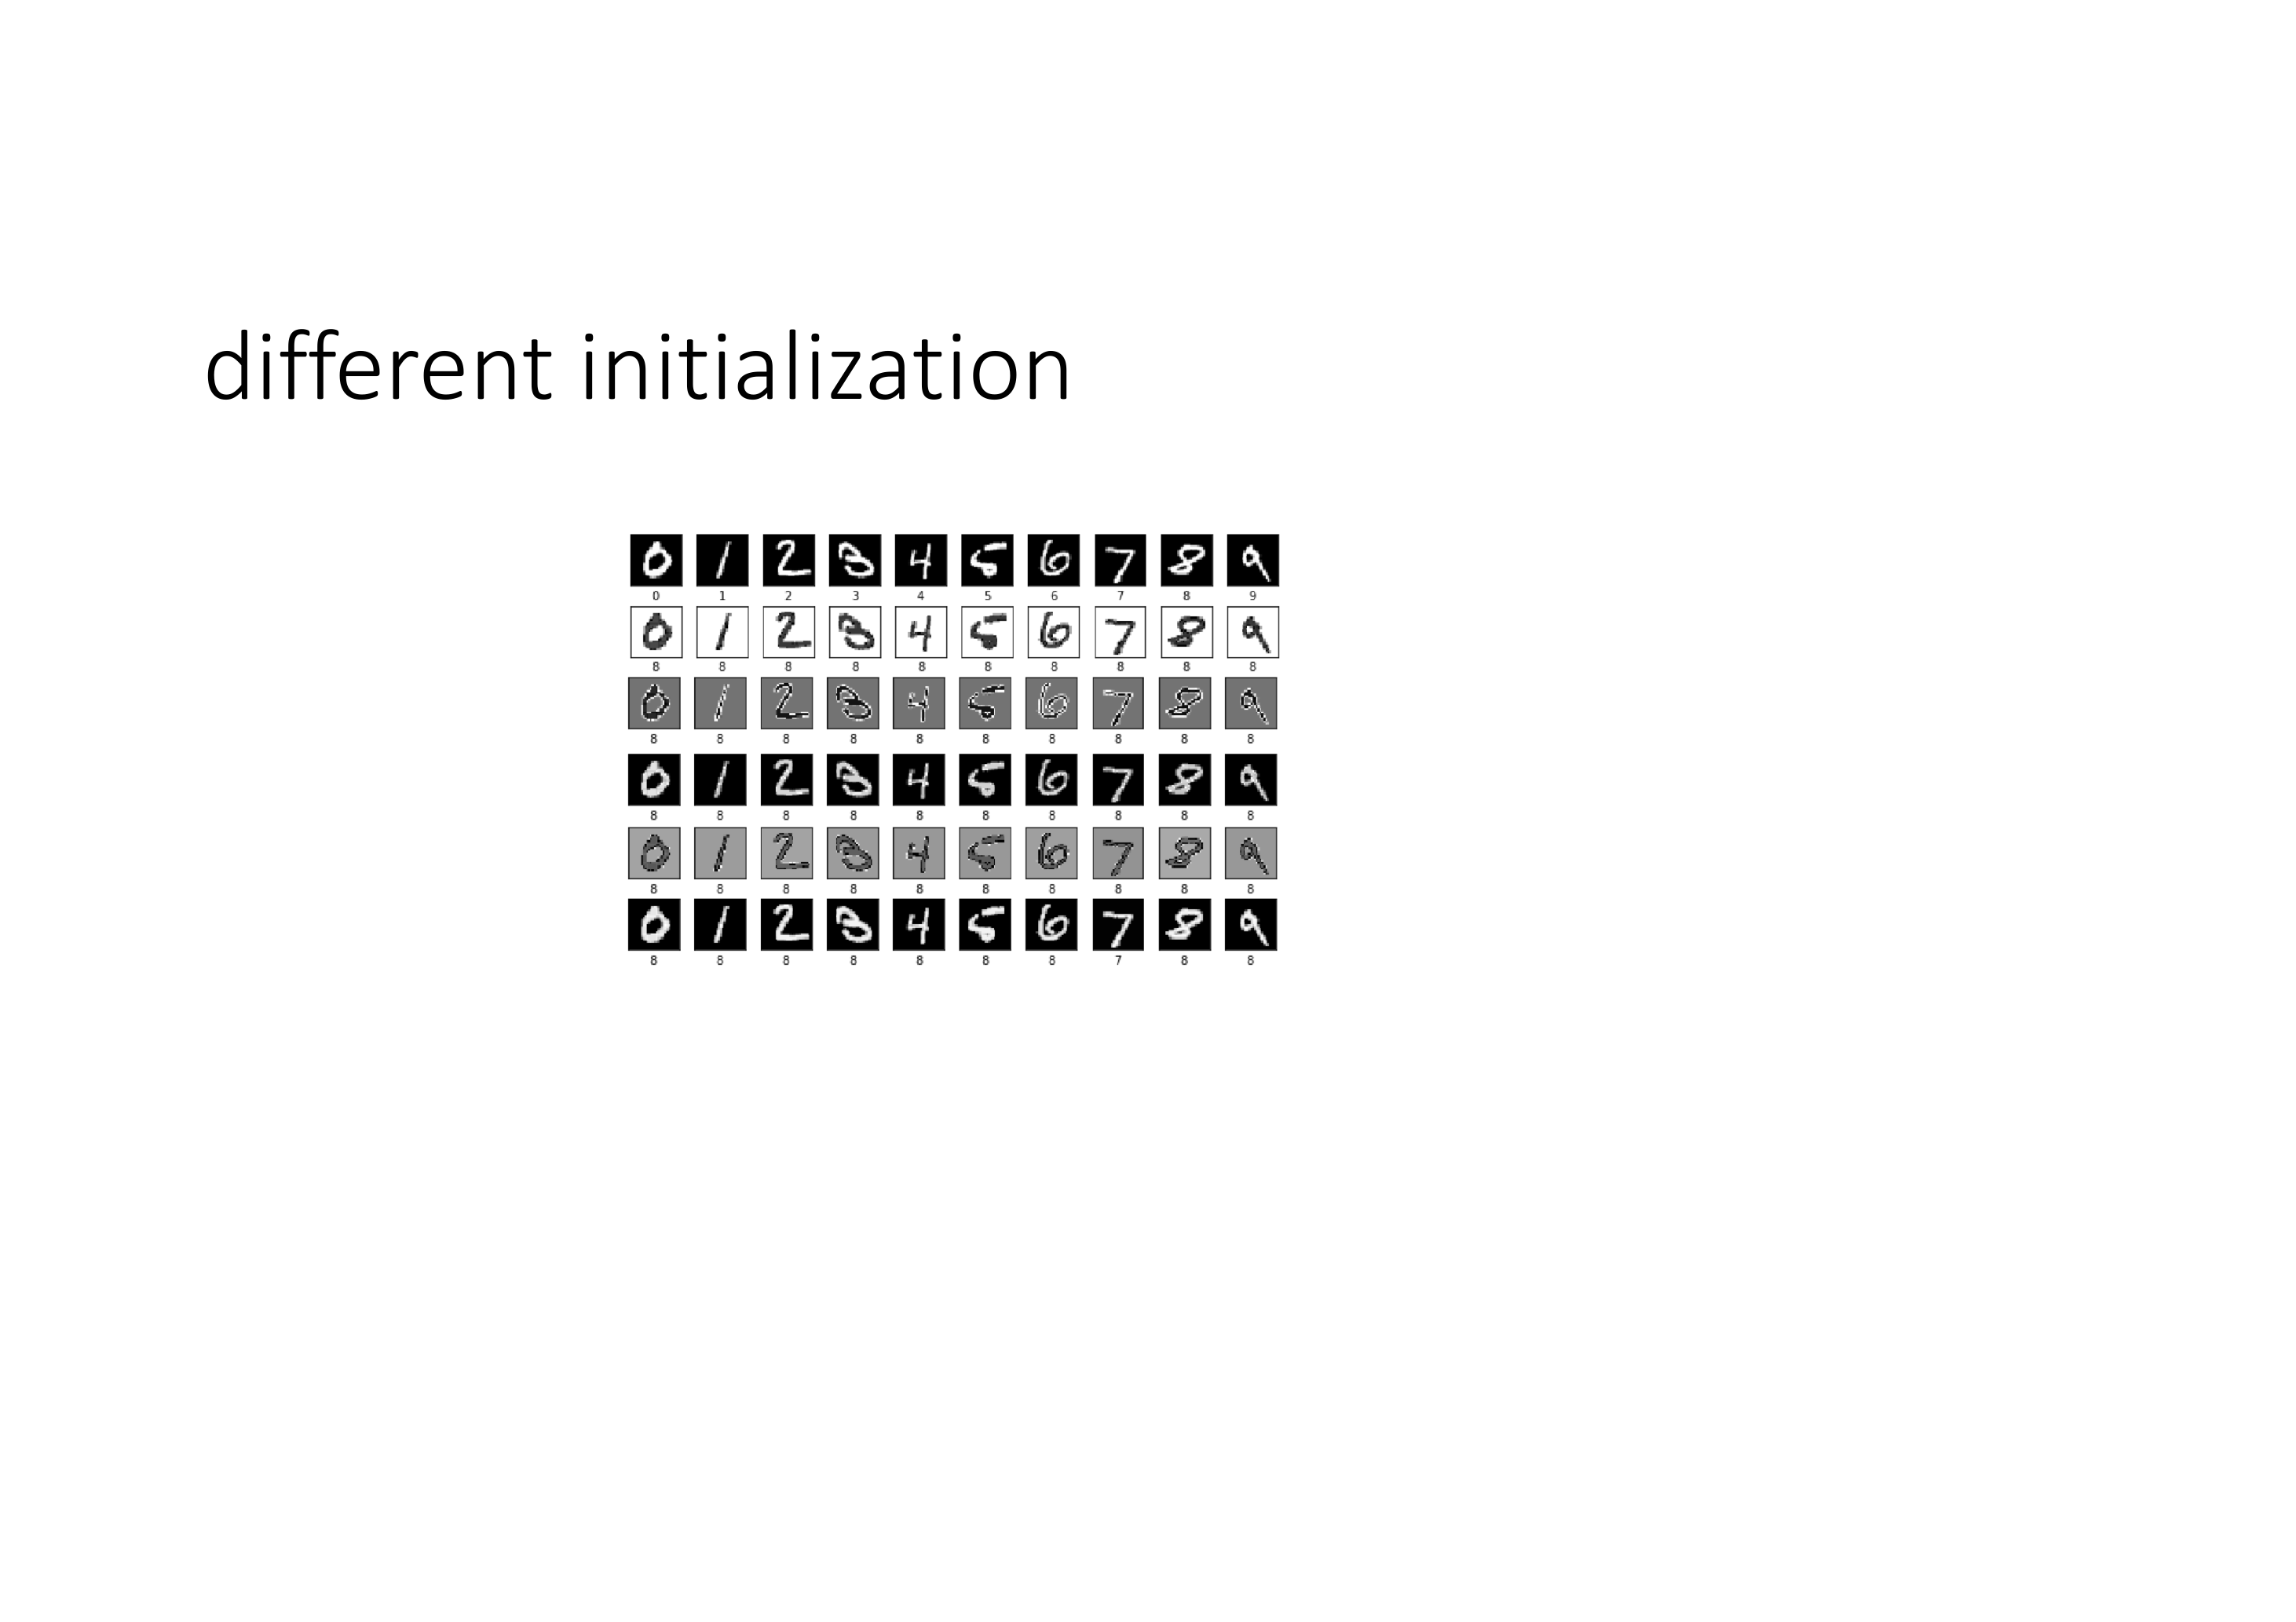}
    \hspace{10px}
    \includegraphics{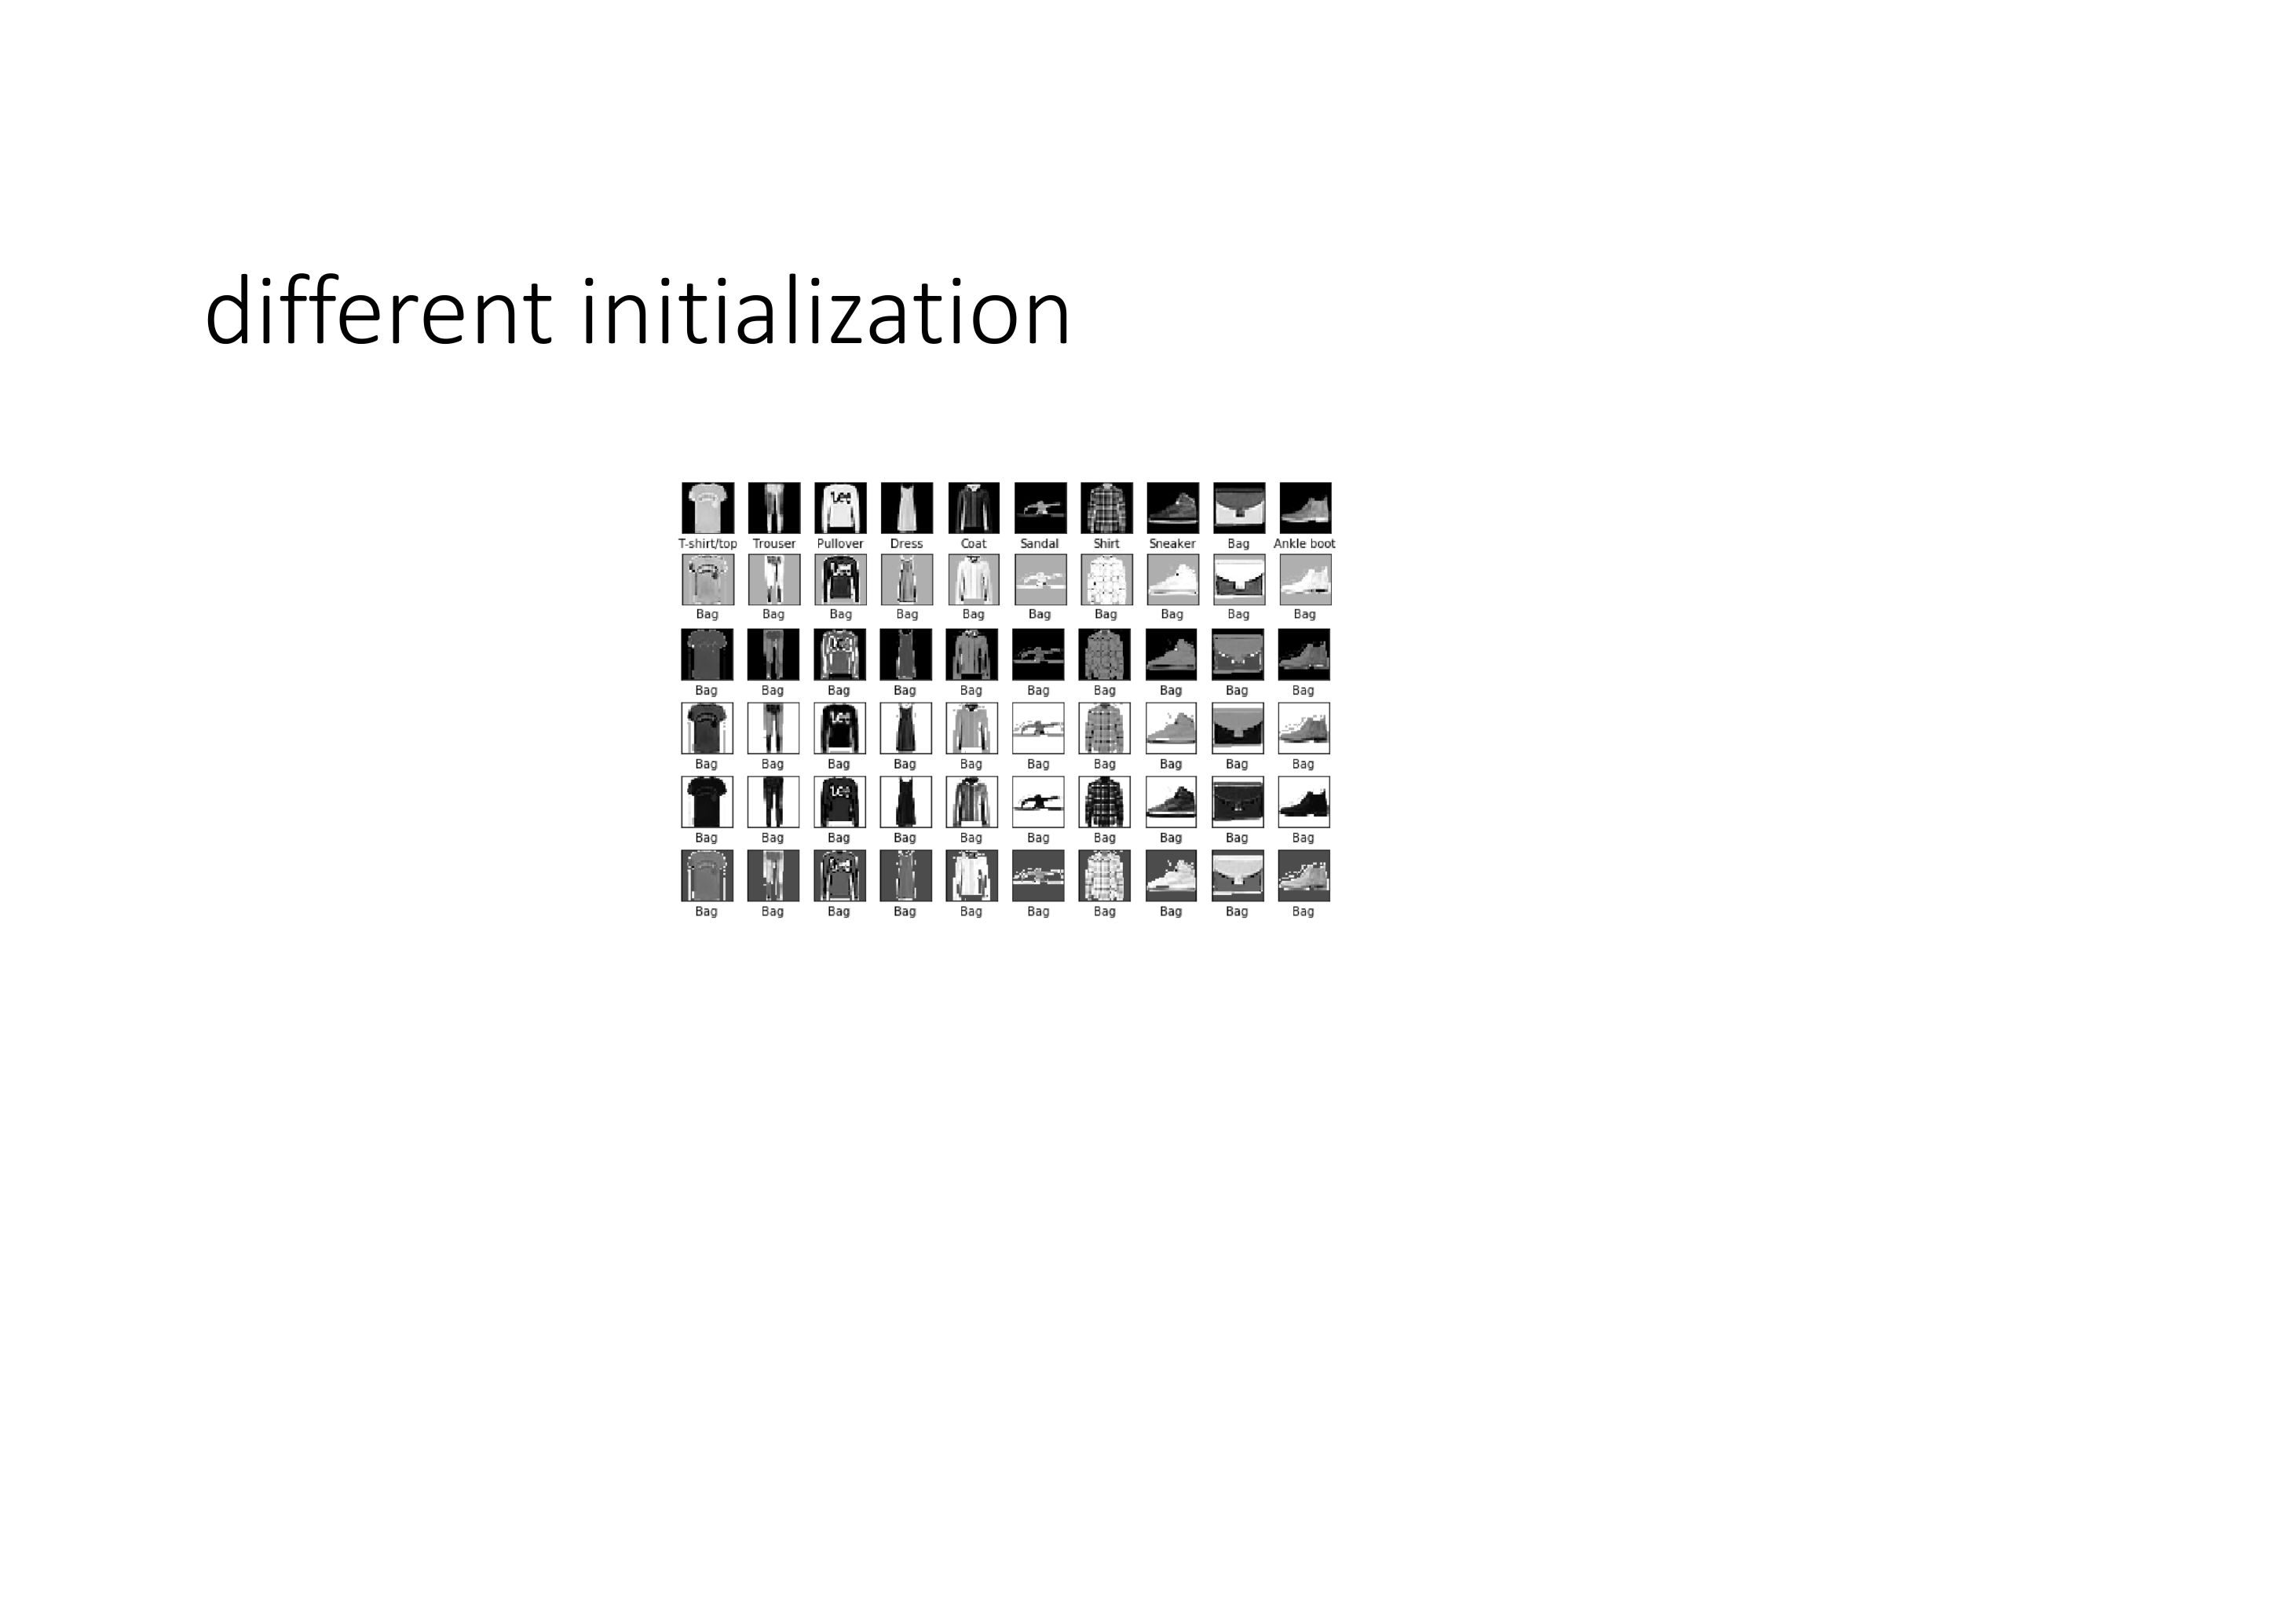}
    \caption{Visual illustration of adversarial examples generated by SPT with different initialization settings. The first row shows the original images selected from MNIST (left) and F-MNIST (right), respectively. The other five rows show the adversarial examples crafted by SPT for different initialization settings, respectively.}
    \label{fig:init_example}
\end{figure*}

\subsection{SPT Adversarial Examples for Different Initialization Settings}

Figure~\ref{fig:init_example} plots the generated SPT adversarial examples against white-box $C_{p}$ with different initial weights. Obviously, the generated SPT adversarial examples vary a lot with different initialization settings.
